# Supplementary material for: Anomalous dynamical scaling determines universal critical singularities
Source: arXiv:2209.02042 ancillary file (2022-10-24)
Supplement: Supplementary file 1 [file SM.pdf]

# Supplemental Material for :"Anomalous dynamical scaling determines universal critical singularities"


Attilio L. Stella,[1,2] Aleksei Chechkin,[3,4,5] and Gianluca Teza[6,a)]

[1)] *Department of Physics and Astronomy, University of Padova, Via Marzolo 8, I-35131 Padova, Italy*
[2)] *INFN, Sezione di Padova, Via Marzolo 8, I-35131 Padova, Italy*
[3)] *Institute of Physics and Astronomy, University of Potsdam, D-14476 Potsdam-Golm, Germany,*
[4)] *Faculty of Pure and Applied Mathematics, Hugo Steinhaus Center, University of Science and Technology, Wyspianskiego 27, 50-370 Wrocław, Poland,*
[5)] *Akhiezer Institute for Theoretical Physics, 61108 Kharkov, Ukraine*
[6)] *Department of Physics of Complex Systems, Weizmann Institute of Science, Rehovot 7610001, Israel*



(Dated: 24 October 2022)



In this supplemental material (SM) we discuss the details of the calculations and results presented in the main text.


## I. LAPLACE'S MAXIMIZATION METHOD

The integral expressing $G(\lambda, t)$ for the scaling observable:

$$G(\lambda, t) \sim \int_{-\infty}^{+\infty} dz\; e^{\lambda t^{\nu} z} f(z) \tag{1}$$

at large $\lambda t^{\nu}$ is controlled by the behavior for large $z$ of the scaling function $f(z)$. We make the ansatz:

$$f(z) \simeq f_{\infty} z^{\psi} e^{-c z^{\delta+1}} \tag{2}$$

for the behavior of $f$ at large $z$, for positive $c$ and $\delta$. Unlike in Eq. (4) of the main text we include here also the asymptotic amplitude $f_{\infty}$ of $f$. According to Laplace's method, if we define $h_{\lambda t^{\nu}}(z) = \lambda t^{\nu} z + \log(f(z))$, the dominant contribution to $\log(G)$ at large $\lambda t^{\nu}$ is then given by:

$$\log(G) \sim h_{\lambda t^{\nu}}(\bar{z}) + \frac{1}{2}\log\left(\frac{2\pi}{h''_{\lambda t^{\nu}}(\bar{z})}\right) + O\left((\lambda t^{\nu})^{-(1+\frac{1}{\delta})}\right) \tag{3}$$

where $\bar{z}$ is the maximum of $h_{\lambda t^{\nu}}$. The second term is the result of Gaussian integration around the maximum. By substituting $\bar{z} \sim (\lambda t^{\nu})^{1/\delta}$ into Eq. 3 we finally get:

$$\log(G) \sim k(\lambda t^{\nu})^{1+\frac{1}{\delta}} + \frac{1}{2}\log\left(\frac{2\pi f_{\infty}^2}{c\delta(\delta+1)}\right) + \frac{2\psi+1-\delta}{2}\log(\bar{z}) \tag{4}$$

where the first term, with the constant $k$, represents the sum of the first two terms reported in Eq.(5) of the main text. The second makes explicit the time independent constant there, which depends on $f_{\infty}$ (see[1] for analogous derivations in the Ising model).

---


[a)] Electronic mail: gianluca.teza@weizmann.ac.il

## II. GENERALIZED MASTER EQUATION FOR CTRW AND THE MITTAG-LEFFLER FUNCTION

We consider a continuous time random walk (CTRW) on a 1-dimensional lattice with spacing $L$ (see[2,3]). The particle hops with some rate (in units $[\text{time}]^{-\alpha}$) $r$ ($l$) to the right (left) nearest neighboring site after a certain time $\tau$ distributed according to a waiting time distribution $\omega(\tau) \sim \tau^{-1-\alpha}$. The probability of observing the particle at a site $i$ at a time $t$ follows the generalized master equation (GME):

$$\partial_t P_i(t) = \int_{-\infty}^{t} d\tau\ K(t-\tau)[rP_{i-1}(\tau) + lP_{i+1}(\tau) - (r+l)P_i(\tau)] \tag{5}$$

where $K(t)$ represents the memory kernel associated to the waiting time distribution by the relation $K(s) = s\omega(s)/(1-\omega(s))$ in Laplace space[4]. The above formulation is equivalent to:

$$\partial_t^\alpha P_i(t) = rP_{i-1}(t) + lP_{i+1}(t) - (r+l)P_i(t) \tag{6}$$

where the operator $\partial_t^\alpha$ represents the fractional Caputo derivative which has the following integral representation[5]:

$$\partial_t^\alpha f(t) = \frac{1}{\Gamma(1-\alpha)} \int_0^t d\tau \frac{\partial_\tau f(\tau)}{(t-\tau)^\alpha} \tag{7}$$

The integral has the shape of a convolution, between the first order time derivative of the function $f$ and the function $t^{-\alpha}$. Therefore, introducing the Laplace transform in time as $f(s) = \int dt\ e^{-st} f(t)$ one finds that the Caputo derivative in Laplace coordinates reads:

$$\int_0^{+\infty} dt\ e^{-st} \partial_t^\alpha f(t) = s^\alpha f(s) - s^{\alpha-1} f(t=0) \tag{8}$$

Hence, the GME of Eq. 6 in Laplace coordinates for time reads:

$$[r+l+s^\alpha]P_i(s) - s^{\alpha-1}\delta_{i,0} = rP_{i-1}(s) + lP_{i+1}(s) \tag{9}$$

where we assumed a Kronecker delta in 0 as initial condition.

The generating function in Laplace coordinate for time can be expressed as $G(\lambda, s) = \sum_i e^{\lambda i} P_i(s)$, which can be shown to satisfy the following equation:

$$G(\lambda, s) = \frac{s^{\alpha-1}}{s^\alpha - \varepsilon_B(\lambda)} \tag{10}$$

where we introduced $\varepsilon_B(\lambda) = r(e^{L\lambda} - 1) + l(e^{-L\lambda} - 1)$, which is exactly the SCGF of the Brownian diffusion (with $\alpha = 1$). The right hand side of the above equation has precisely the form of the Laplace representation of the one parameter Mittag-Leffler function $E_\alpha(\varepsilon_B(\lambda)t^\alpha)$, which can be written in terms of an infinite series as[6]:

$$E_\alpha(z) = \sum_{k=0}^{\infty} \frac{z^k}{\Gamma(1+\alpha k)} \tag{11}$$

for any $z \in \mathbb{C}$ and $\alpha \in \mathbb{C}$ with positive real part, and $\Gamma$ represents the Gamma function. The asymptotic behavior on the real axis has an exponential dependence for positive and a power-law for negative arguments. Specifically we have for some $N \in \mathbb{N}$:

$$E_\alpha(x) \sim \frac{1}{\alpha} e^{x^{1/\alpha}} - \sum_{k=1}^{N} \frac{1}{\Gamma(1-\alpha k)} \frac{1}{x^k} + O(x^{-N-1}) \text{ for } x \to +\infty \tag{12}$$

$$E_\alpha(x) \sim -\sum_{k=1}^{N} \frac{1}{\Gamma(1-\alpha k)} \frac{1}{x^k} + O(x^{-N-1}) \text{ for } x \to -\infty \tag{13}$$

implying that the asymptotic behaviors of the generating function are $\sim e^{\varepsilon_B(\lambda)^{1/\alpha} t}$ (resp. $-1/\varepsilon_B(\lambda)t^\alpha$) for positive (resp. negative) values of $\varepsilon_B(\lambda)$.

## III. FRACTIONAL DRIFT DIFFUSION EQUATION AND THE M-WRIGHT FUNCTION

In the continuum limit of the spacing of the discrete lattice going to zero, Eq. 6 provides the fractional drift diffusion equation (which reduces to plain diffusion in the unbiased $r = l$ case). This can be seen easily by symmetrizing ($p = (r + l)/2$) and anti-symmetrizing ($q = (r - l)/2$) the rates to separate the diffusing from the drifting part. Given that $r = p + q$ and $l = p - q$. the master equation can be easily rewritten as:

$$\partial_t^\alpha P_i(t) = -2qL\frac{P_{i+1}(t) - P_{i-1}(t)}{2L} + pL^2\frac{P_{i-1}(t) + P_{i+1}(t) - 2P_i(t)}{L^2} \tag{14}$$

where we recognize on the r.h.s. a first and second order discrete central derivatives of the probability. Taking the continuum limit by sending the spacing of the lattice $L \to 0$, allows to extend the discrete coordinate $iL \to x$ with continuous $x \in \mathbb{R}$, gives $pL^2 \to D$ and $2qL \to K$ as diffusion and drift constants, and naturally defines the probability density function

$$p(x,t) = \lim_{L\to 0}\frac{1}{L}P_i(t) \tag{15}$$

Combining everything one finally finds that $p$ satisfies the fractional drift diffusion equation:

$$\partial_t^\alpha p(x,t) = -K\partial_x p(x,t) + D\partial_x^2 p(x,t) \tag{16}$$

which in the unbiased case ($r = l$ implies $K \equiv 0$) reduces to the plain fractional diffusion equation. In units in which $D = 1$, in the long time limit the fractional diffusion equation (without drift) is exactly solved by $p(x,t) = t^{-\nu}M_\nu(x/t^\nu)$ where $M_\nu$ is the M-Wright function which has the following asymptotic representation for large values[7]:

$$M_\nu(z) \sim a(\nu)|\nu z|^{\frac{\nu-1/2}{1-\nu}}e^{-b(\nu)|\nu z|^{1/(1-\nu)}} \tag{17}$$

where we introduced $z = x/t^\nu$ and with $\nu = \alpha/2$, and the (positive) coefficients $a(\nu)$ and $b(\nu)$ have the form

$$a(\nu) = \frac{1}{\sqrt{2\pi(1-\nu)}},\ b(\nu) = \frac{1-\nu}{\nu} \tag{18}$$

The solution to the biased case described by Eq. 16 has been found exactly in[8] as a solution to a continuum model of time-fractional kinetic equation. Applying the Laplace transform to Eq. 16

$$p(x,s) = \int_0^\infty e^{-st}p(x,t)dt \tag{19}$$

and solving the equation in Laplace space separately for $x < 0$ and $x > 0$, we get with $p(x,s) \to 0$ at $x \to \pm\infty$

$$p(x,s) = \frac{s^{\alpha-1}}{\sqrt{K^2 + 4Ds^\alpha}}\exp\left(\frac{Kx}{2D} - |x|\frac{\sqrt{K^2+4Ds^\alpha}}{2D}\right). \tag{20}$$

Expanding around $s = 0$ for $0 < \alpha < 1$ allows us to characterize the long-time behavior, which is clearly different for positive and negative values of $x$. For $x > 0$ we get the following representation in Laplace and time coordinates

$$p(x,s) \sim \frac{s^{\alpha-1}}{K}e^{-\frac{xs^\alpha}{K}} \ \leftrightarrow\ p(x,t) \sim \frac{1}{Kt^\alpha}M_\alpha\left(\frac{x}{Kt^\alpha}\right) \text{ for } x \geq 0 \tag{21}$$

while for $x < 0$ we obtain

$$p(x,s) \sim \frac{s^{\alpha-1}}{K}e^{\frac{Kx}{D}} \ \leftrightarrow\ p(x,t) \sim \frac{t^{-\alpha}}{K\Gamma(1-\alpha)}e^{\frac{Kx}{D}} \text{ for } x < 0 \tag{22}$$

It is clear how in the infinite time limit the probability of being on the negative axis becomes identically zero. The probability is therefore concentrated on the positive axis, following a distribution modulated by the M-Wright function.

This asymmetric shape can be shown to be directly related with the singularities of the associated $\varepsilon(\lambda)$ and the flat region between them. The PDF of Eq. 20 is an exact solution in Laplace coordinates of time for Eq. 16. We can use it to find the Laplace transform of the generating function $G(\lambda, s) = \int_{-\infty}^{+\infty} dx\, e^{\lambda x} p(x, s)$. Straightforward calculations yield:

$$G(\lambda, s) = \frac{s^{\alpha-1}}{s^{\alpha} - (K\lambda + D\lambda^2)} \tag{23}$$

Here we recognize the Laplace representation of the Mittag-Leffler function, implying that the generating function in the time domain reads:

$$G(\lambda, t) = E_{\alpha}[(K\lambda + D\lambda^2)t^{\alpha}] \tag{24}$$

which has an exponential (power-law) asymptotic behavior for positive (negative) arguments. The SCGF is found taking the limit

$$\varepsilon(\lambda) = \lim_{t\to\infty} \frac{1}{t} \log G(\lambda, t) = \begin{cases} (K\lambda + D\lambda^2)^{1/\alpha} & \lambda \le -K/D \text{ and } \lambda \ge 0 \\ 0 & -K/D < \lambda < 0 \end{cases} \tag{25}$$

A proper connection with the SCGF of the CTRW presented in the main text can be established assuming a local detailed balance relation[9–11] linking the rates with the external force $F$ acting on the particle, assumed to have a certain mass $m$ and to be subject to a fractional friction $\gamma_{\alpha}$, as defined in[8]. The fractional and drift diffusion coefficients are parametrized as:

$$K = \frac{F}{m\gamma_{\alpha}} \ , \ D = \frac{k_B T}{m\gamma_{\alpha}} \tag{26}$$

where $k_B$ is the Boltzmann constant and $T$ the temperature (the diffusion form is determined by Einstein's relation). At mesoscopic level, the rates appearing in the CTRW must satisfy locally the detailed balance relation

$$r/l = e^{\frac{FL}{k_B T}} \tag{27}$$

where we remind that $L$ is the spacing of the discrete lattice. Straightforward algebra shows that

$$-K/D = L^{-1} \log l/r \equiv \lambda_0 \tag{28}$$

## IV. RATE FUNCTION OF AN ANOMALOUS CTRW DIFFUSION WITH BIAS

In the biased ($r > l$) CTRW presented in the manuscript we have shown that the SCGF has the form

$$\varepsilon(\lambda) = \begin{cases} \varepsilon_B(\lambda)^{1/\alpha} & \lambda \le \lambda_0 \text{ and } \lambda \ge 0 \\ 0 & \lambda_0 < \lambda < 0 \end{cases} \tag{29}$$

where $\varepsilon_B(\lambda) = r(e^{\lambda} - 1) + l(e^{-\lambda} - 1)$ and $\lambda_0 = L^{-1} \log l/r$. The SCGF is convex and differentiable for $0 < \alpha < 1$. A large deviation principle is satisfied given the existence of the SCGF, and thanks to the aforementioned properties we can apply Gartner-Ellis theorem to obtain the rate function modulating the probability of observing a certain "velocity" $v = x/t$:

$$I(v) = \sup_{\lambda \in \mathbb{R}} [v\lambda - \varepsilon(\lambda)] \tag{30}$$

Solving the supremum problem implies inverting the differential equation $\partial_\lambda\varepsilon(\lambda) = v$, which cannot be done analytically for every $\alpha$. However, one can obtain the rate function in a parametric form defining $v_\lambda \equiv \partial_\lambda\varepsilon(\lambda)$:

$$\{v_\lambda, I_\lambda\} \equiv \{\partial_\lambda\varepsilon(\lambda), v\partial_\lambda\varepsilon(\lambda) - \varepsilon(\lambda)\} \tag{31}$$

Analyzing this parametric form one can understand many details of the rate function. First, we see that the rate function is zero for $v = 0$, consistently with the idea that a canonical current cannot be defined in an anomalously diffusing process. Moreover, one sees tat the values $\lambda > 0$ determine the positive branch of the rate function, while $\lambda < \lambda_0$ determines the negative one. The flat area between $\lambda_0$ and 0 is instead responsible for a singularity of the first derivative of $I(v)$ at $v = 0$. Therefore, in order to determine the behavior of the rate function around zero for positive (negative) values one needs to study the behavior of $\varepsilon(\lambda)$ for $\lambda \to 0^+$ ($\lambda \to \lambda_0^-$).

Let us study the positive branch first. Here we know that $\varepsilon(\lambda) \sim (r-l)^{1/\alpha}\lambda^{1/\alpha}$ for $\lambda \to 0^+$, which implies:

$$v_\lambda = \partial_\lambda\varepsilon(\lambda) \sim \tfrac{1}{\alpha}(r-l)^{1/\alpha}\lambda^{1/\alpha-1} \tag{32}$$

$$I_\lambda = \lambda\partial_\lambda\varepsilon(\lambda) - \varepsilon(\lambda) \sim \tfrac{1-\alpha}{\alpha}(r-l)^{1/\alpha}\lambda^{1/\alpha} \; . \tag{33}$$

Solving for $\lambda$ the first equation and substituting in the second one yields:

$$I_\lambda \sim v_\lambda^{\frac{1}{1-\alpha}} \tag{34}$$

Let us now address the negative branch. As already mentioned, we need to look at the behavior of the SCGF for $\lambda \to \lambda_0^-$, which is found to be $\varepsilon(\lambda) \sim (r-l)^{1/\alpha}(\lambda_0-\lambda)^{1/\alpha}$. This provides us with:

$$v_\lambda = \partial_\lambda\varepsilon(\lambda) \sim -\frac{1}{\alpha}(r-l)^{1/\alpha}(\lambda_0-\lambda)^{1/\alpha-1} \tag{35}$$

$$I_\lambda = \lambda\partial_\lambda\varepsilon(\lambda) - \varepsilon(\lambda) \sim \frac{1-\alpha}{\alpha}(r-l)^{1/\alpha}(\lambda_0-\lambda)^{1/\alpha} + \\ -\frac{\lambda_0}{\alpha}(r-l)^{1/\alpha}(\lambda_0-\lambda)^{1/\alpha-1} \tag{36}$$

The first term on the right hand side of the equation for $I_\lambda$ is sub-leading with respect to the second. Therefore, we can conclude that

$$I_\lambda \sim \lambda_0 v_\lambda \tag{37}$$

for the negative branch of the rate function (remember $\lambda_0 < 0$ so $I_\lambda > 0$ for negative $v_\lambda$), which as we can see is not dependent on $\alpha$.

## V. FLUCTUATION THEOREM

The symmetry of the SCGF allows for a straightforward and exact validation of the fluctuation theorem. It states that the probability of observing a positive fluctuation of the observable, the velocity in our case, divided by the probability of observing a negative fluctuation of the same magnitude increases exponentially both with time and the magnitude of the observable. Formally:

$$\frac{p(v,t)}{p(-v,t)} = e^{\text{const.}\cdot vt} \tag{38}$$

for some positive constant with a positive bias. Given that the probability is modulated asymptotically by a rate function as $p(v,t) \sim e^{-tI(v)}$, the above relation takes the form

$$\frac{p(v,t)}{p(-v,t)} = e^{-t(I(v)-I(-v))} \tag{39}$$

Expressing the rate function as the Legendre-Fenchel transform of the SCGF thanks to the Gartner-Ellis theorem[12,13], we can express:

$$\begin{aligned} I(-v) &= \sup_{\lambda\in\mathbb{R}}[-v\lambda - \varepsilon(\lambda)] = \\ &= \sup_{\lambda'\in\mathbb{R}}[v\lambda' - \varepsilon(-\lambda')] = \\ &= \sup_{\lambda'\in\mathbb{R}}[v\lambda' - \varepsilon(\lambda' + \lambda_0)] = \\ &= -v\lambda_0 + \sup_{\lambda\in\mathbb{R}}[v\lambda - \varepsilon(\lambda)] = -v\lambda_0 + I(v) \end{aligned} \tag{40}$$

where we exploited the symmetry of the SCGF $\varepsilon(-\lambda) = \varepsilon(\lambda + \lambda_0)$. Substituting this exact result in the equation for the ratio of the probability finally yields:

$$\frac{p(v,t)}{p(-v,t)} = e^{-t\lambda_0 v} \tag{41}$$

implying a validity of the fluctuation theorem with const. $= -\lambda_0 > 0$.


[1] A. Bruce, "Critical finite-size scaling of the free energy," Journal of Physics A: Mathematical and General **28**, 3345 (1995).

[2] E. W. Montroll and G. H. Weiss, "Random walks on lattices. ii," Journal of Mathematical Physics **6**, 167–181 (1965).

[3] V. Kenkre, E. Montroll, and M. Shlesinger, "Generalized master equations for continuous-time random walks," Journal of Statistical Physics **9**, 45–50 (1973).

[4] R. Metzler and J. Klafter, "The random walk's guide to anomalous diffusion: a fractional dynamics approach," Physics Reports **339**, 1–77 (2000).

[5] A. Carpinteri and F. Mainardi, *Fractals and fractional calculus in continuum mechanics*, Vol. 378 (Springer, 2014).

[6] R. Gorenflo, A. A. Kilbas, F. Mainardi, and S. V. Rogosin, *Mittag-Leffler functions, related topics and applications* (Springer, 2020).

[7] F. Mainardi, A. Mura, and G. Pagnini, "The M-Wright function in time-fractional diffusion processes: a tutorial survey," International Journal of Differential Equations **2010** (2010), 10.1155/2010/104505.

[8] A. V. Chechkin and R. Klages, "Fluctuation relations for anomalous dynamics," Journal of Statistical Mechanics: Theory and Experiment **2009**, L03002 (2009).

[9] S. Katz, J. L. Lebowitz, and H. Spohn, "Phase transitions in stationary nonequilibrium states of model lattice systems," Phys. Rev. B **28**, 1655–1658 (1983).

[10] G. Teza, S. Iubini, M. Baiesi, A. L. Stella, and C. Vanderzande, "Rate dependence of current and fluctuations in jump models with negative differential mobility," Physica A: Statistical Mechanics and its Applications **552**, 123176 (2020), tributes of Non-equilibrium Statistical Physics.

[11] G. Teza, *Out of equilibrium dynamics: from an entropy of the growth to the growth of entropy production*, Ph.D. thesis, University of Padova (2020).

[12] J. Gärtner, "On large deviations from the invariant measure," Theory of Probability & Its Applications **22**, 24–39 (1977), https://doi.org/10.1137/1122003.

[13] R. S. Ellis, "Large deviations for a general class of random vectors," The Annals of Probability **12**, 1–12 (1984).
